# Supplementary material for: Robust Aggregation for Adaptive Privacy Preserving Federated Learning in Healthcare
Source: arXiv:2009.08294 source file (2020-09-17)
Supplement: Supplementary file 1 [file css-appendix.tex]

\section{Aggregation Strategies Performance}

Along the experiments presented in section 4, we have looked at many other different scenarios, corresponding to different training data partitioning, hyper-parameters and clients configurations. For having a better reference when interpreting the results, we provide below the results for four aggregation strategies when no privacy preserving mechanism has been used and no bad clients interfere in the training process. We use the same two medical datasets, same hyper-parameters and the same number of federated clients. The results show that, in general, Byzantine-robust aggregation schemes don't significantly impact the training performance. However, MKRUM in the case of the Heart Disease dataset decreases the performance of the global model.

\begin{figure*}[!htb]
    \centering
    \includegraphics[width=1.0\textwidth]{./pics/robust_agg_only.png} % heartNoByz.png
    \caption[Diabetes and Heart Disease classification task performance of different FL aggregation schemes]{Appendix-I (aggregation schemes performance): It shows the results from the four aggregation schemes while performing the Diabetes Prediction (left) and Heart Disease (right) classification task without bad clients when no privacy preserving technique being used.}
    \label{fig:heart}
\end{figure*}
